# Supplementary material for: Position Paper: Agent AI Towards a Holistic Intelligence
Source: arXiv:2403.00833 source file (2024-02-28)
Supplement: Supplementary file 1 [file 8_appendix.tex]

\section{Ablations and Analysis}
\label{sec:discussion}

\textbf{Comparisons with GPT-4V} In Figure \ref{fig:gpt4v-comparison}, we show how our model has the capability to output low-level action predictions, while GPT-4V is unable to consistently output low-level controls.  While our model is able to output precise movements and actions, GPT-4V is largely relies on outputting high-level text.

\textbf{Effects of Agent Pretraining}  In Table \ref{tab:gaming_baselines} and Table \ref{tab:healthcare_baselines}, we demonstrate the effectiveness of our agent pre-training strategy compared to training from scratch and training against an equivalent visual-language baseline.
